# Supplementary material for: Implementation of Analytical Jacobian and Chemical Explosive Mode Analysis (CEMA) in OpenFOAM
Source: arXiv:2205.07416 source file (2022-05-16)
Supplement: Supplementary file 1 [file Appendix1.tex]

\chapter{Manipulate chemical mechanisms using Cantera}

Requires: Cantera software package

\todo{APPENDIX TO BE ADDED DURING REVISION PHASE}

% \section{First Section}

% The first section of the appendix goes here. 

% \section{Second Section}

% The second section of the appendix goes here. 

\section{Convert CHEMKIN-II to .cti format using Cantera}

\section{Generate analytical Jacobian src code using PyJac}
